# Supplementary material for: Byzantine Consensus is \Theta(n^2): The Dolev-Reischuk Bound is Tight even in Partial Synchrony! [Extended Version]
Source: arXiv:2208.09262 source file (2022-09-06)
Supplement: Supplementary file 1 [file Dolev_Reischuk_bound_complete.tex]

\section{Generalized Dolev-Reischuk Bound} \label{section:generalized_dolev}

Dolev-Reischuk lower bound~\cite{Dolev1985} says that any Byzantine consensus protocol operating in a partially synchronous environment has $\Omega(f^2)$ communication complexity, where $f$ represents the number of tolerated Byzantine processes.
Importantly, Dolev and Reischuk consider the Byzantine consensus problem satisfying \emph{strong validity:} if all correct processes propose the same value, then only that value can be decided by a correct process.
As \name does not satisfy strong validity, it does not (technically speaking) match the Dolev-Reischuk lower bound.
In this section, we show that \name is indeed optimal, as we generalize the Dolev-Reischuk bound for consensus protocols \emph{not} satisfying strong validity.
Our proof is strongly inspired by~\cite{AbrahamBlog}.

We consider a partially synchronous consensus protocol $\mathsf{Consensus}$ ensuring both agreement and termination (see \Cref{section:introduction}).
A process $P_i$ proposes its value to $\mathsf{Consensus}$ from a predefined set $\mathbb{I}$, and it decides its value from a predefined set $\mathbb{O}$.
We denote by $I_i$ the input value of process $P_i$ (i.e., its proposal), and by $O_i$ the output value of process $P_i$ (i.e., its decision).

% , that has to ensure at least both agreement and termination, i.e. every process $p$ proposes its input value from an allowed set $\mathbb{V}_I^p$ and all correct processes eventually decide a common output value in an allowed set $\mathbb{V}_O$. Since we do not want to consider a trivial solution, where all correct processes decide a value hard-coded in advance, protocol $\Pi$ has to ensures additional non-trivial property. This property is quasi-systematically defined in accordance with the inputs of the correct processes (since we assume that processes might fail, we only care about input of correct processes). This motivates the next definition of \emph{configuration input}.

% At the beginning of each execution, each process is labelled as either \emph{good} or \emph{bad}.
% If a process is good, the process follows its protocol; otherwise, it may deviate from its protocol. 
An \emph{input configuration} of an execution of $\mathsf{Consensus}$ is $\mathit{input} = \{(p, I_p) \text{ with } p \text{ is correct}\}$: an input configuration consists of input values of all correct processes.
We denote by $\mathcal{I}$ is the set of all input configurations. 
% An execution of $\Pi$ is said to \emph{start} with an input configuration $i = \{(p, I_p) \text{ with } p \text{ is good and } I_p \in \mathbb{V}_{I}^p\}$ if every good process $p$ proposes $I_p \in \mathbb{V}_{I}^p$ with $(p,I_p) \in i$. 
The validity property satisfied by $\mathsf{Consensus}$ is defined with a function $\mathsf{Validity}$ that maps an input configuration $\mathit{input}$ into a set of possible output values $\mathsf{Validity}(\mathit{input})$.
The $\mathsf{Validity}$ function satisfies the following two properties:
\begin{compactitem}
    \item \emph{Feasibility:} For any two input configurations $\mathit{input}_1, \mathit{input}_2$ such that $\mathit{input}_1 \subseteq \mathit{input}_2$, \\$\mathsf{Validity}(\mathit{input}_2) \subseteq \mathsf{Validity}(\mathit{input}_1)$.
    
    Let us explain why we assume this property.
    Suppose that the property does not hold.
    Hence, there exists a value $v \in \mathsf{Validity}(\mathit{input}_2)$ such that $v \notin \mathsf{Validity}(\mathit{input}_1)$.
    Therefore, there exists an execution $E$ in which (1) the input configuration is $\mathit{input}_2$, and (2) $v \in \mathsf{Validity}(\mathit{input}_2)$ is decided.
    If every process that is labelled correct in $\mathit{input}_2$ and not labelled correct in $\mathit{input}_1$ behaves exactly as in execution $E$ in an execution with the input configuration $\mathit{input}_1$, correct processes will decide $v \notin \mathsf{Validity}(\mathit{input}_1)$ in the execution.
    Thus, no consensus protocol satisfies such a validity property.
    
    \item \emph{Non-triviality:} $\underset{\mathit{input} \in \mathcal{I}}{\bigcap} \mathsf{Validity}(\mathit{input}) = \emptyset$.
    
    We define the non-triviality property in order to avoid trivial solutions to the problem.
    Indeed, if $v \in \underset{\mathit{input} \in \mathcal{I}}{\bigcap} \mathsf{Validity}(\mathit{input})$, a protocol in which all correct processes immediately decide $v$ solves the problem.
\end{compactitem}

\begin{theorem} [Generalized Dolev-Reischuk lower bound]
The communication complexity of $\mathsf{Consensus}$ is $\Omega(f^2)$.
% The worst-case communication complexity of a consensus protocol is $\Omega(f^2)$.%$(\lceil f/2 \rceil)^2$%Let $\Pi$ be distributed protocol among a set $\Psi$ of processes, where every correct process $p \in \Psi$ proposes an input value in a set $\mathbb{V}^{p}_{I}$ and can decide an output value in a set  $\mathbb{V}_O$. Let assume $\Pi$ ensures both Termination and Agreement with $f$-resiliency and $o(f^2)$ worst-case communication complexity. Then it exists a process $p \in \Psi$, a value $z \in \mathbb{V}_O$ and a set of executions execution $E^{*}_{p,z} = \{e^{*}_{p,x,z} | x \in \mathbb{V}^p_{I}\}$ of $\Pi$ where process $p$ is correct, proposes an allowed input $x \in \mathbb{V}^p_{I}$ and decides $z \in \mathbb{V}_O$ without receiving any message.
\end{theorem}

\begin{proof}
We prove the theorem by contradiction.
Therefore, let the communication complexity of $\mathsf{Consensus}$ be $o(f^2)$.

\smallskip
\noindent \textbf{Part 1.} \emph{There exists a process $P_i$ that (if correct) decides some value $z$ without receiving any message.}
% \textbf{Part 1. By agreement, termination and sub-quadratic complexity, it exists a correct process $p$ that always decide the same value without receiving any message} \newline
\smallskip
\\ Let us partition all processes into two disjoint groups: (1) group $U$, where $|U| = n - \lceil f/2 \rceil$, and (2) group $V$, where $|V| = \lceil f/2 \rceil$.
Let $E$ be an execution of $\mathsf{Consensus}$ in which all processes in $U$ are correct, and all processes in $V$ are Byzantine and silent. 
All processes in $U$ eventually decide the same value $z \in \mathbb{O}$.

Since correct processes send $\lceil f/2 \rceil^2$ messages in $E$ (otherwise, the communication complexity of $\mathsf{Consensus}$ would not be $o(f^2)$), there exists a process $P_i$ that receives less than $\lfloor f / 2 \rfloor$ messages in $E$.
We denote by $U' \subset U$ the set of processes that have sent messages to process $P_i$ in $E$; note that $|U'| \leq \lfloor f / 2 \rfloor$.

Now, for every value $x \in \mathbb{I}$, we construct an execution $E^{*}_{x,z}$ of $\mathsf{Consensus}$:
\begin{compactitem}
    \item All processes in the $U \setminus{U'}$ set are correct.
    Moreover, process $P_i$ is correct and proposes $x \in \mathbb{I}$.
    
    \item Processes in the $V \setminus{\{P_i\}}$ set are faulty and silent, i.e., they do not send any message. 
    
    \item Processes in the $U'$ set are faulty, and behave exactly as they do in $E$, except that they do not send any message to $P_i$.
    
    \item Execution $E^{*}_{x,z}$ is indistinguishable from $E$ to processes in the $U \setminus{U'}$ set.
\end{compactitem}
Note that $E^{*}_{x,z}$ has (at most) $f - 1$ faulty processes ($\lceil f / 2 \rceil - 1$ faults in the group $V$ and $\lfloor f / 2 \rfloor $ faults in the group $U'$).
Moreover, all processes in the $U \setminus{U'}$ set decide $z$ (since they do not distinguish $E^{*}_{x,z}$ from $E$ until their decision).
Finally, $P_i$ does not receive any message in $E^{*}_{x,z}$; moreover, $P_i$ decides $z$ in $E^{*}_{x,z}$ (because of the termination and agreement properties satisfied by $\mathsf{Consensus}$). 

Hence, there exists a process $P_i$, a value $z \in \mathbb{O}$, and a set of executions $E^{*}_{z} = \{E^{*}_{x,z} | x \in \mathbb{I}\}$ of $\mathsf{Consensus}$ such that $P_i$ is correct, it proposes a value $x$ and it decides $z$ after some finite time without receiving any message.

\smallskip
\textbf{Epilogue.}
We divide all input configurations into $\mathcal{I}_{P_i \in C}$ and $\mathcal{I}_{P_i \notin C}$, where $\mathcal{I}_{P_i \in C}$ (resp., $\mathcal{I}_{P_i \notin C}$) is the set of input configurations in which $P_i$ is (resp., is not) labelled as correct.

Consider an input configuration $\mathit{input} \in \mathcal{I}$.
If $\mathit{input} \in \mathcal{I}_{P_i \notin C}$, we note $\mathit{enriched}(\mathit{input}) = \mathit{input} \cup \{(P_i, x_{\mathit{input}}) \}$ with an arbitrary value $x_{\mathit{input}} \in \mathbb{I}$. 
If $\mathit{input} \in \mathcal{I}_{P_i \in C}$, $\mathit{enriched}(\mathit{input}) = \mathit{input}$. 
Trivially, $\mathit{input} \subseteq \mathit{enriched}(\mathit{input})$.

Let us construct an execution $E_{\mathit{input}}$ with the input configuration $\mathit{enriched}(\mathit{input})$:
\begin{compactitem}
    \item Process $P_i$ does not distinguish $E_{\mathit{input}}$ from an execution $E^*_{x, z}$ (recall that, in partial synchrony, messages can be delayed).
\end{compactitem}
Therefore, $P_i$ decides $z$ in $E_{\mathit{input}}$.
Furthermore, $z \in \underset{\mathit{input} \in \mathcal{I}}{\bigcap} \mathsf{Validity}(\mathit{enriched}(\mathit{input}))$.
Because of the feasibility property of $\mathsf{Validity}$ and the fact that $\mathit{input} \subseteq \mathit{enriched}(\mathit{input})$, for every $\mathit{input} \in \mathcal{I}$, $\mathsf{Validity}(\mathit{enriched}(\mathit{input})) \subseteq \mathsf{Validity}(\mathit{input})$.
\\Hence, $\underset{\mathit{input} \in \mathcal{I}}{\bigcap} \mathsf{Validity}(\mathit{enriched}(\mathit{input})) \subseteq \underset{\mathit{input} \in \mathcal{I}}{\bigcap} \mathsf{Validity}(\mathit{input})$, which implies that \\$z \in \underset{\mathit{input} \in \mathcal{I}}{\bigcap} \mathsf{Validity}(\mathit{input})$.
Therefore, the $\mathsf{Validity()}$ function does not satisfy non-triviality, thus a contradiction.
\end{proof}

We emphasize that both weak~\cite{Milosevic2009} and binary~\cite{MostefaouiMR15} validity properties satisfy both feasibility and non-triviality, and are, thus, covered by the generalized Dolev-Reischuk bound. 
Therefore, \name is an optimal consensus protocol satisfying weak validity, and \sname is an optimal consensus protocol satisfying binary validity.\footnote{Recall that the original bound shows that \sname is optimal in solving Byzantine consensus with strong validity.}
